# Supplementary material for: Online Linear Regression in Dynamic Environments via Discounting
Source: arXiv:2405.19175 source file (2024-05-29)
Supplement: Supplementary file 1 [file appendix.tex]

%auto-ignore
\documentclass[paper]{subfiles}
\begin{document}

\appendix

\subfile{./Appendices/discounted-vaw.tex}
    \subfile{./Appendices/small-loss.tex}
\subfile{./Appendices/lb.tex}
\subfile{./Appendices/tuning.tex}
    \subfile{./Appendices/experts.tex}
\subfile{./Appendices/strongly-adaptive.tex}
\subfile{./Appendices/baby-comparison.tex}
\subfile{./Appendices/lemmas.tex}

\end{document}
